# Supplementary material for: Towards The Implicit Bias on Multiclass Separable Data Under Norm Constraints
Source: arXiv:2603.22824 source file (2026-03-24)
Supplement: Supplementary file 1 [file appendix.tex]

% 重置定理、引理等计数器，使其从1开始
\newpage
\setcounter{theorem}{0}
\setcounter{lemma}{0}
\setcounter{corollary}{0}
\setcounter{remark}{0}
